# Supplementary material for: An optimal-transport finite-particle method for mass diffusion
Source: arXiv:2305.05315 source file (2023-05-09)
Supplement: Supplementary file 1 [file Appendix.tex]

\begin{appendix}

\section{Elements of optimal transportation theory}\label{WUv9vk}

{\color{blue} MO: Shorten.}

For completeness, in this appendix we collect basic elements of optimal transportation theory that underpin the present work. A complete account of the theory may be found, e.~g., in \cite{fedeli2017geometrically, Villani2003, Daneri:2014100}.

Let $\Omega \subseteq \mathbb{R}^d$ an open convex set and let $\mathscr{P}(\Omega)$, the space of Borel probability measures on $\Omega$. If $\mu \in \mathscr{P}(\Omega)$ and $\varphi: \Omega \rightarrow \Omega$ is a Borel map, $\varphi_{\#}\mu \in \mathscr{P}(\Omega)$ denotes the \emph{push-forward} of $\mu$ through $\varphi$, defined by
\begin{equation}
    \varphi_{\#}\mu(B)
    :=
    \mu(\varphi^{-1}(B)) \quad \text{for every } B \text{ Borel }
    \in \mathscr{P}(\Omega).
\end{equation}
Let $\pi^i, \,\, i = 1 \dots n$ be the canonical projection operator from a product space $\Omega \times \dots \times \Omega$ onto $\Omega$,
\begin{equation}
    \pi^i(z_1,\dots,z_n) := z_i .
\end{equation}
Given $\mu_1 \in \mathscr{P}(\Omega)$ and $\mu_2 \in \mathscr{P}(\Omega)$ the class $\Gamma(\mu_1,\mu_2)$ of \emph{transport plans} or \emph{couplings} between $\mu_1$ and $\mu_2$ is defined as
\begin{equation}
    \Gamma(\mu_1,\mu_2) := \{ {\gamma} \in \mathscr{P}(\Omega \times \Omega) \}: \pi^1_{\#}{\gamma} = \mu_1, \pi^2_{\#}{\gamma} = \mu_2\}.
\end{equation}
We denote by $\mathscr{P}_2(\Omega)$ the space of Borel probability measures with finite second moment: $\mu \in \mathscr{P}(\Omega)$ belongs to $\mathscr{P}_2(\Omega)$ iff:
\begin{equation}
    \int_{\Omega}| x - x_{0}|^2 {\rm d}\mu(x)
    <
    +\infty, \quad \text{for some (and thus every) point }
    x_{0} \in \Omega.
\end{equation}
For every pair of measures $\mu,\nu \in \mathscr{P}_2(\Omega)$ we consider the transport cost
% consider the Kantorovich problem for the cost $|\cdot - \cdot|^2$
\begin{equation}\label{wdist}
    d_W^2(\mu,\nu)
    :=
    \min \left \{ \int_{\Omega\times \Omega} |x-y|^2 {\rm d} \gamma(x,y) :
    \gamma \in \Gamma(\mu,\nu)\right \}.
\end{equation}
By the direct method of calculus of variations, the minimum problem (\ref{wdist}) admits at least a solution. The minimum value $d_W(\mu,\nu)$ defines a distance between the measures $\mu,\nu \in \mathscr{P}_2(\Omega)$ and the metric space $(\mathscr{P}_2(\Omega),d_W)$ is referred to as the ($L^2$-) \emph{Wasserstein space} on $\Omega$. We denote by $\mathscr{P}_2^a(\Omega)$ the subset of $\mathscr{P}_2(\Omega)$ formed by the absolutely continuous measures with respect to the Lebesgue measure,
\begin{equation}
    \mathscr{P}_2^a(\Omega)
    :=
    \{ \mu \in \mathscr{P}_2(\Omega) : \mu  \ll \mathcal{L}^d \}.
\end{equation}
The following result establishes the existence and uniqueness of optimal transport plans induced by maps, or \emph{optimal transport maps}, got the case in which the initial measure $\mu$ belongs to $\mathscr{P}_2^a(\Omega)$.

\begin{thm}[Existence and uniqueness of optimal transport maps \cite{Brenier1991, KnottSmith1984} ] For any $\mu \in \mathscr{P}_2^a(\Omega)$ and $\nu \in \mathscr{P}_2(\Omega)$, the Kantorovich optimal transport problem (\ref{wdist}) has a unique solution $\gamma$, which is concentrated on the graph of a transport map, namely, the unique minimizer of Monge's optimal transport problem
\begin{equation}
    \min \left \{ \int_{\Omega} | x - \varphi(x)|^2 {\rm d}\mu(x) \,: \, \varphi_{\#}\mu = \nu  \right \}.
\end{equation}
The map $\varphi$ is cyclically monotone and there exists a convex function $\phi: \Omega \rightarrow \mathbb{R}$ such that $\varphi(x) = \nabla \phi(x)$ for $\mu-a.e. \, x \in \Omega$.
\end{thm}

We also recall that the manifold $\mu \in \mathscr{P}_2(\Omega)$ can be endowed with a canonical differential structure. In particular, the tangent space to $\mathscr{P}_2(\Omega)$ at the point $\mu$ is defined as
\begin{equation}
    \textnormal{Tan}_{\mu}\mathscr{P}_2(\Omega)
    :=
    \overline{ \{ \xi: \xi = \nabla \eta, \, \eta \in
    C_c^{\infty}(\Omega)\}}^{L^2(\Omega, \mu)} ,
\end{equation}
where the elements of $\textnormal{Tan}_{\mu}\mathscr{P}_2(\Omega)$ may be regarded as velocity fields.  Indeed, for any absolutely continuous curve $t \mapsto \mu_t \in \mathscr{P}_2(\Omega)$ with $\mu_0 = \mu$, there exists a unique $\xi \in \textnormal{Tan}_{\mu}\mathscr{P}_2(\Omega)$ such that
\begin{equation}
    \left. \frac{\partial }{\partial t}\mu_t \right |_{t =0}
    +
    \nabla \cdot (\mu \xi) = 0 \quad \text{in} \,\,\mathcal{D}'(\Omega).
\end{equation}
In particular, if $\mu_t \in \mathscr{P}_2^a(\Omega)$, and $\rho_t$ is its density with $\rho_\infty = \rho$, then
\begin{equation}
    \left. \frac{d}{dt} \right |_{t=0} \int_{\Omega} \rho_t(x)\eta(x) dx
    =
    \int_{\Omega} \xi(x) \cdot \nabla \eta(x) \rho(x)dx ,
\end{equation}
for all test functions $\eta \in \mathcal{D}(\Omega)$. Thus, changes in densities in $\mathscr{P}_2^a(\Omega)$ are to be regarded as mass fluxes induced by velocity fields.

We also recall the following differentiation formula. Let $b > a$, $\rho_a$, $\rho_b \in \mathscr{P}_2^a(\Omega)$ and let $\rho_t \in \mathscr{P}_2^a(\Omega)$, $t \in [a,b]$, be such $\rho(\cdot,a) = \rho_a$, $\rho(\cdot,b) = \rho_b$ and
\begin{equation}
    \frac{\partial \rho_t}{\partial t} + \nabla \cdot (\rho_t \xi) = 0 ,
\end{equation}
for some $C^1$, globally bounded, velocity field $\xi$. Then \cite{Villani2003},
\begin{equation}\label{diffeWdist}
    \frac{{\rm d}}{{\rm d}t} d_W^2(\rho_a,\rho_t) \restriction_{t=b}
    =
    2 \int_{\Omega} \langle x - \varphi_{\rho_b},
    \xi(x)\rangle {\rm d}\rho_b(x)
\end{equation}
where $\varphi_{\rho_b}$ is the unique optimal transport map between $\rho_a$ and $\rho_b$.

%\section{Differentiation of $\mathscr{U}$ }

We conclude by showing that the first variation in $\mathscr{P}_2(\Omega)$ of the entropy
\begin{equation}
    S(\rho_{k+1}) = \int_{\Omega} \rho_{k+1}\log \rho_{k+1} \, dx
\end{equation}
gives (\ref{eq:TD:DFmin}) and (\ref{eq:TD:RVD3}). Thus, let $\xi \in  C^{\infty}_c({\Omega})$ be a smooth vector field with compact support. Define the variation $y = \psi(x,t) = \psi_{t}(x)$ as
\begin{equation}\label{variations}
    \partial_{t} y = \xi(y), \,\, y(0) = x .
\end{equation}
Let $\rho_{t}$ be the pushforward measure of $\rho_{k+1}$ by $\psi_t$, i.~e.,
\begin{equation}\label{push_density}
    \int_{\Omega} \rho_t(x) \eta(x) \, dx
    =
    \int_{\Omega} \rho_{k+1} \eta(\psi_t(x)) \,dx ,
\end{equation}
for all $\eta \in C^{\infty}_{0}(\Omega)$.  Since $\psi_t$ is regular, (\ref{push_density}) is equivalent to the relation between densities
\begin{equation}\label{density_relation}
    \big( {\rm det}(\nabla\psi_t) \, \rho_t \big) \circ \psi_t = \rho_{k+1}.
\end{equation}
In particular,
\begin{equation}
    \int_{\Omega} \rho_t \, dx = \int_{\Omega} \rho_{k+1} \, dx ,
\end{equation}
and $\rho_t$ is in $\mathscr{P}_2(\Omega)$. In addition, we have
\begin{equation}
    \int_{\Omega} \rho_t(x) \log(\rho_t(x)) \, dx %\overset{(\ref{push_density})}
    {=}
    \int_{\Omega}
    \rho_{k+1}(x)\log(\rho_t(\psi_t(x))) \, dx %\overset{(\ref{density_relation})}
    {=}
    \int_{\Omega} \rho_{k+1} \log \left( \frac{\rho_{k+1}(x)}{\text{det}\nabla \psi_{t}(x)} \right) \, dx ,
\end{equation}
and
\begin{equation}
    \frac{1}{t} \left (  S (\rho_t) - S (\rho_{k+1}) \right )
    =
    -
    \frac{1}{t} \int_{\Omega} \rho_{k+1}(x)\log(\text{det}\nabla \psi_t(x)) \, dx.
\end{equation}
Write
\begin{equation}
    J_{\psi_t} := \text{det}\nabla \psi_t .
\end{equation}
Then, we have
\begin{equation}
\begin{split}
    \frac{{\rm d}}{{\rm d}t}\left [ J_{\psi_t} \right ]|_{t = 0}
    & =
    \left. \left [ \frac{\partial \, J_{\psi_t}}{\partial \, \nabla \psi_t } \,
    {\cdot}
    \, \frac{\partial \, \nabla \psi_t }{\partial t}  \right ] \right |_{t=0}
    =
    \left. \left [ J_{\psi_t} (\nabla \psi_t)^{-T} \, {\cdot} \, \nabla \left(\frac{\partial \psi_t}{\partial t} \right)
    \right ] \right |_{t = 0}
    \\ & =
    \left. \left [ J_{\psi_t} (\nabla \psi_t)^{-T} \, {\cdot} \, \nabla \xi \right ] \right |_{t = 0}
    =
    \text{I} \, {\cdot} \, \nabla \xi = \nabla \cdot \xi ,
\end{split}
\end{equation}
where we have used that $\psi(x,0) = \text{id}$. Taking the limit $t \rightarrow 0$, we find
\begin{equation}
    \frac{{\rm d}}{{\rm d}t} S (\rho_t)|_{t = 0}
    =
    -\int_{\Omega}\rho_{k+1}(x)\nabla \cdot \xi(x) \, dx,
\end{equation}
as advertised.

\section{Euler-Lagrange equations of the JKO functional}\label{8heHO0}

Thus, taking variations we obtain (cf.~Appendix, eq.~(\ref{diffeWdist}), also \cite{Villani2003})
\begin{equation}\label{eq:TD:DFmin}
\begin{split}
    \langle DF(\varphi_{k\to k+1}), \xi_{k+1} \rangle
    & =
    \frac{1}{t_{k+1}-t_k}
    \int_\Omega \langle x-\varphi_{k+1\to k}(x), \xi_{k+1}(x) \rangle
    \rho_{k+1}(x) \, dx
    \\ & -
    \int_\Omega \kappa (\log\rho_{k+1} + 1) \nabla\cdot(\rho_{k+1}\xi_{k+1}) \, dx ,
    \\ & =
    \frac{1}{t_{k+1}-t_k}
    \int_\Omega \langle x-\varphi_{k+1\to k}(x), \xi_{k+1}(x) \rangle
    \rho_{k+1}(x) \, dx
    \\ & +
    \int_\Omega \kappa \nabla \rho_{k+1}\cdot \xi_{k+1} \, dx ,
\end{split}
\end{equation}
where we write
\begin{equation}
    \varphi_{k+1\to k}
    =
    \varphi_{k\to k+1}^{-1} ,
\end{equation}
and the variations satisfy the boundary condition
\begin{equation}
    \xi_{n+1} \cdot n = 0 .
\end{equation}
Enforcing stationarity for all admissible variations yields
\begin{equation}\label{eq:TD:RVD3}
    \rho_{k+1}(x)
    \frac{x-\varphi_{k+1\to k}(x)}{t_{k+1}-t_k}
    =
    -
    \kappa \nabla \rho_{k+1}(x) ,
\end{equation}
which is indeed a time discretization of (\ref{rVre5S}).

\end{appendix}
